# Supplementary material for: Test-Time Alignment for Tracking User Interest Shifts in Sequential Recommendation
Source: arXiv:2504.01489 source file (2025-04-02)
Supplement: Supplementary file 1 [file 6_appendix.tex]

\appendix

\section{Hyperparameters}
In all methods and experiments, we conducted a grid search on the hyperparameters to pick the setting with the best results. The hyperparameters and other reproducibility information for \ourname\ setting on the ML-1M dataset are provided in Table~\ref{hyper}. All methods were implemented using PyTorch~\cite{paszke2019pytorch}.
\begin{table}[htb]
\centering
\caption{Hyperparameters and other reproducibility information for \ourname.}
\begin{tabular}{l|r}
\hline Hyper-parameter & Value \\
\hline \hline Optimizer & Adam~\cite{kingma2014adam}\\
Data Splitting Strategy & Leave-One-Out~\cite{wong2015performance} \\
Number of Epoch & $500$ \\
Evaluation Step & $10$ \\
Early Stopping Step & $3$ \\
Indicator Metric & NDCG@$10$ \\
\hline
Learning Rate & $0.01$ \\
Embedding Dimension & $64$ \\
State Dimension & $32$ \\
Convolution Width & $4$ \\
Training Batch Size & $4096$ \\
Inference Batch Size & $40960000$ (Full Dataset) \\
Layer Num & $1$ \\
Dropout & $0.2$ \\
$M$: Training Step during Testing & $1$ \\
$\alpha$: Learning Rate during Testing & $0.05$ \\
$\mu_1^{\text{train}}$: Training weight for $\mathcal{L}_{\text{ssl1}}$  & $\{0.01, \mathbf{0.1}, 1, 10\}$ \\
$\mu_2^{\text{train}}$: Training weight for $\mathcal{L}_{\text{ssl2}}$  & $\{0.01, 0.1, \mathbf{1}, 10\}$ \\
$\mu_1^{\text{test}}$: Testing weight for $\mathcal{L}_{\text{ssl1}}$  & $\{1e^{-5}, 1e^{-4}, \mathbf{1e^{-3}}, 1e^{-2}, 1e^{-1}\}$ \\
$\mu_2^{\text{test}}$: Testing weight for $\mathcal{L}_{\text{ssl2}}$ & $\{1e^{-5}, 1e^{-4}, 1e^{-3}, \mathbf{1e^{-2}}, 1e^{-1}\}$ \\

\hline
\end{tabular}
\label{hyper}
\end{table}
